# Supplementary material for: PAD: Patch-Agnostic Defense against Adversarial Patch Attacks
Source: arXiv:2404.16452 source file (2024-04-25)
Supplement: Supplementary file 1 [file X_suppl.tex]

\clearpage
\setcounter{page}{1}
\maketitlesupplementary

%=========================================================
\section{Morphological Operations in Fusion Block}
\label{sec:morphological}
After applying the adaptive thresholding, we perform morphological operations on the heat map with the main purpose of removing isolated background points and purifying the patch area. For an input image with dimensions $w\times h\times c$, we set the adaptive base kernel size as follows:
\begin{equation}
k_{base}=\frac{min(w,h)}{\delta }\times\frac{min(w,h)}{\delta } ,
\end{equation}
where $\delta$ is a fixed hyperparameter that we set to 80 in our implementation. To minimize the impact on the integrity of the patch area, we adopt a progressive strategy. The initial opening operation uses a kernel of size $k_{base}\times2$, followed by a closing operation with a kernel size of $k_{base}$, and finally a second opening operation with a kernel size of $k_{base}\times3$. 
We visualize each step of the morphological operation process, as shown in Figure \ref{fig:morph}. As shown in the examples, small noise pixels are initially removed during the first opening operation. Subsequently, the closing operation fills in small holes within the patch region, preventing disconnected areas from being eroded in the subsequent opening operation. Finally, the larger kernel size in the opening operation effectively eliminates spikes or small bridges, resulting in a more accurate and complete patch region. The consecutive application of these morphological operations optimizes and refines the patch localization results.

\begin{figure}[h]
    \centering
    \includegraphics[width=0.48\textwidth]{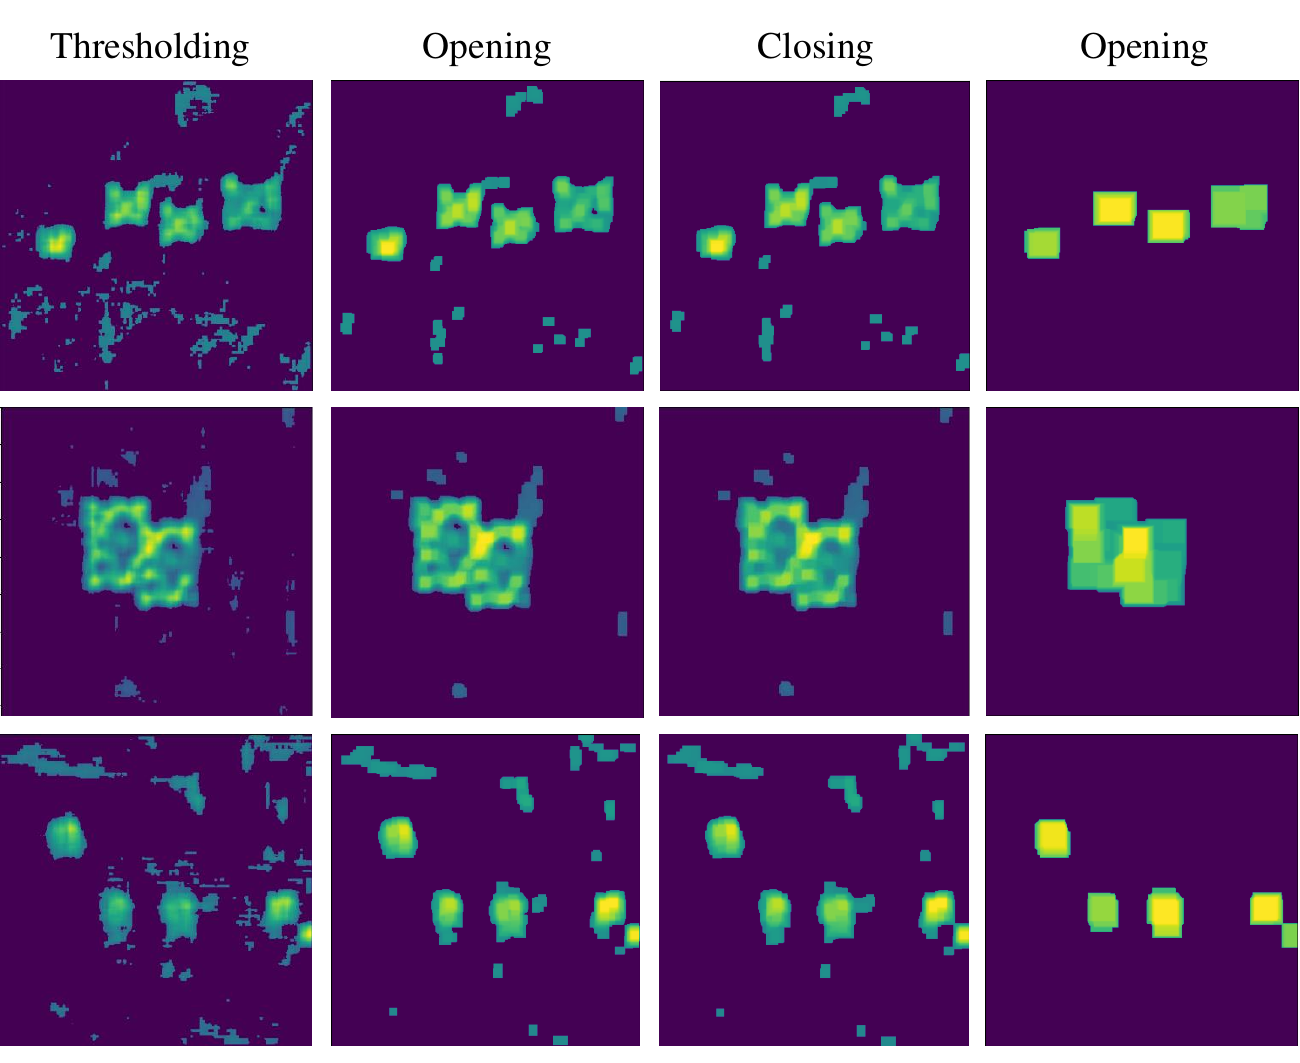}
    \caption{Visualization examples of morphological operations.}
    \label{fig:morph}
\end{figure}

%=========================================================
\section{More About Evaluation on Digital Attacks}

%----------------------------------
\subsection{Defense performance against more attacks}
We conduct additional defense experiments against more state-of-the-art physical patch attack methods \cite{hu2022adversarial}\cite{huang2023t} on different datasets. As shown in Table \ref{tab:r-more}, PAD achieves the best performance against all of them. Among them, experiments against AdvTexture and T-SEA are conducted on YOLOv2, and the rest are conducted on Faster R-CNN. The experimental results demonstrate the generalizability of PAD in diverse detection scenarios.
   
\begin{table}[h]
\centering
\caption{mAP (\%) under more attacks on different datasets.}
\label{tab:r-more}
\resizebox{0.48\textwidth}{!}{%
\begin{tabular}{c|c|cccccc}
\hline
Attack                 & Dataset                                                & Undefended & LGS   & SAC   & Jedi  & PZ\cite{xu2023patchzero}    & \textbf{PAD}   \\ \hline
\begin{tabular}[c]{@{}c@{}}AdvTexture\\ \cite{hu2022adversarial}\end{tabular}            & Inria                                                  & 43.51      & 75.26 & 59.08 & 68.88 & -     & \textbf{79.83} \\ \hline
\multirow{2}{*}{\begin{tabular}[c]{@{}c@{}}T-SEA\\\cite{huang2023t}\end{tabular} } & Inria                                                  & 17.05      & 35.15 & 17.60 & 40.22 & -     & \textbf{74.93} \\ \cline{2-8} 
                       & \begin{tabular}[c]{@{}c@{}}COCO-\\ Person\end{tabular} & 10.56      & 13.33 & 10.59 & 15.32 & -     & \textbf{30.93} \\ \hline
Dpatch                 & COCO                                                   & 29.1       & 40.7  & 44.1  & 38.5  & -     & \textbf{45.1}  \\ \hline
Masked PGD             & VOC                                                    & 10.90      & 61.53 & 62.81 & 60.79 & 66.10 & \textbf{67.12} \\ \hline
\end{tabular}%
}
% \vspace{-1.2em}
\end{table}

%----------------------------------
\subsection{Defense performance on other detectors}
In addition to the experimental results on Faster R-CNN, YOLOv3, and YOLOv5s listed in Table 1 of the main paper, we also conduct defense performance evaluations on YOLOv2 \cite{redmon2017yolo9000} and YOLOv8n \cite{YOLOv8} with the same setting. The detailed results are presented in Table \ref{tab:yolov2v8}.

\begin{table*}[t]
\centering
\caption{mAP(\%) on YOLOv2 and YOLOv8n. The best performance is \textbf{bolded}, and the suboptimal performance is \underline{underlined}.}
\label{tab:yolov2v8}
\resizebox{\textwidth}{!}{%
\begin{tabular}{c|c|c|ccccccccc}
\hline
Detector                 & Defense             & Clean          & OBJ            & OBJ-CLS        & Upper          & P1             & P2             & P3             & P4             & P5             & P6             \\ \hline
\multirow{5}{*}{YOLOv2}  & Undefended          & \textit{90.13} & \textit{3.71}  & \textit{10.48} & \textit{20.99} & \textit{12.07} & \textit{60.50} & \textit{24.50} & \textit{49.23} & \textit{33.93} & \textit{21.10} \\
                         & LGS (WACV19)        & 89.28          & 5.27           & 46.63          & 55.75          & 20.43          & 61.59          & 27.62          & 60.88          & 38.41          & 27.30          \\
                         & SAC (CVPR22)        & \textbf{90.11} & {\ul 60.48}    & {\ul 67.90}    & {\ul 68.20}    & 17.70          & 24.75          & 24.75          & {\ul 64.58}    & 35.05          & 22.69          \\
                         & Jedi (CVPR23)       & 89.01          & 19.30          & 63.26          & 52.03          & {\ul 26.30}    & {\ul 62.90}    & {\ul 49.56}    & 57.69          & {\ul 48.26}    & {\ul 53.77}    \\
                         & \textbf{PAD (Ours)} & {\ul 89.77}    & \textbf{76.79} & \textbf{82.92} & \textbf{81.33} & \textbf{35.79} & \textbf{79.71} & \textbf{75.00} & \textbf{80.88} & \textbf{78.23} & \textbf{71.88} \\ \hline
\multirow{5}{*}{YOLOv8n} & Undefended          & \textit{96.42} & \textit{56.74} & \textit{75.30} & \textit{65.77} & \textit{68.48} & \textit{50.89} & \textit{51.78} & \textit{65.81} & \textit{51.64} & \textit{50.06} \\
                         & LGS (WACV19)        & {\ul 96.60}    & 47.52          & 82.57          & 82.00          & 68.14          & 51.41          & 53.11          & {\ul 79.42}    & 62.40          & 64.30          \\
                         & SAC (CVPR22)        & 96.42          & {\ul 81.92}    & {\ul 86.95}    & {\ul 84.59}    & {\ul 69.86}    & 51.03          & 51.80          & 78.19          & 53.51          & 50.95          \\
                         & Jedi (CVPR23)       & \textbf{96.64} & 57.63          & 64.35          & 58.13          & 69.85          & {\ul 66.20}    & {\ul 66.94}    & 65.90          & {\ul 64.20}    & {\ul 69.51}    \\
                         & \textbf{PAD (Ours)} & 96.40          & \textbf{87.53} & \textbf{87.69} & \textbf{88.92} & \textbf{70.73} & \textbf{74.84} & \textbf{78.68} & \textbf{85.37} & \textbf{81.51} & \textbf{77.25} \\ \hline
\end{tabular}%
}
\end{table*}

From the experimental results, it can be observed that, consistent with the results on Faster R-CNN, YOLOv3, and YOLOv5s, our PAD achieves the best defense performance on YOLOv2 and YOLOv8n as well. 
PAD demonstrates a considerable improvement in mean average precision (mAP) compared to suboptimal state-of-the-art methods when defending against different types of adversarial patches while maintaining a similar clean performance.

%----------------------------------
\subsection{Ablation study for patch inpainting}
After obtaining an accurate patch mask, PAD employs a simple inpainting method: replacing the patch region with black pixels, which is consistent with \cite{liu2022segment,chiang2021adversarial}. To validate the effectiveness of this inpainting approach, we compare it with another inpainting method: the coherence transport-based inpainting method (inpaintBCT) \cite{bornemann2007fast}, which is used in Jedi \cite{tarchoun2023jedi}. We evaluate the defense performance using these two inpainting methods on different detectors, as shown in Table \ref{tab:ablation-inpaint}.

\begin{table*}[]
\centering
\caption{mAP (\%) of inpainting-ablated PAD under different adversarial patch attacks. The best performance is \textbf{bolded}.}
\label{tab:ablation-inpaint}
\resizebox{\textwidth}{!}{%
\begin{tabular}{c|l|ccccccccc}
\hline
Detector                                                                & \multicolumn{1}{c|}{Defense} & OBJ            & OBJ-CLS        & Upper          & P1             & P2             & P3             & P4             & P5             & P6             \\ \hline
\multirow{2}{*}{\begin{tabular}[c]{@{}c@{}}Faster\\ R-CNN\end{tabular}} & PAD-inpaintBCT               & 82.60          & \textbf{89.44} & 85.84          & \textbf{71.50} & 83.05          & 83.14          & 84.75          & 84.79          & 79.64          \\
                                                                        & PAD-black                    & \textbf{86.80} & 87.80          & \textbf{88.95} & 68.40          & \textbf{87.81} & \textbf{85.00} & \textbf{87.56} & \textbf{89.21} & \textbf{83.23} \\ \hline
\multirow{2}{*}{YOLOv2}                                                 & PAD-inpaintBCT               & 74.51          & 82.07          & 79.45          & 23.73          & 76.17          & 74.25          & 78.12          & 76.67          & 64.71          \\
                                                                        & PAD-black                    & \textbf{76.79} & \textbf{82.92} & \textbf{81.33} & \textbf{35.79} & \textbf{79.71} & \textbf{75.00} & \textbf{80.88} & \textbf{78.23} & \textbf{71.88} \\ \hline
\multirow{2}{*}{YOLOv3}                                                 & PAD-inpaintBCT               & 84.49          & 89.98          & 87.19          & \textbf{83.26} & 82.90          & 83.73          & 86.28          & 84.22          & 80.53          \\
                                                                        & PAD-black                    & \textbf{85.84} & \textbf{91.06} & \textbf{88.56} & 78.00          & \textbf{87.38} & \textbf{87.46} & \textbf{89.13} & \textbf{87.76} & \textbf{86.13} \\ \hline
\multirow{2}{*}{YOLOv5s}                                                & PAD-inpaintBCT               & 78.73          & 83.22          & 78.66          & \textbf{45.21} & 58.28          & 66.02          & 66.91          & 58.57          & 54.15          \\
                                                                        & PAD-black                    & \textbf{84.01} & \textbf{83.62} & \textbf{84.54} & 42.01          & \textbf{58.38} & \textbf{69.87} & \textbf{78.97} & \textbf{67.31} & \textbf{61.08} \\ \hline
\multirow{2}{*}{YOLOv8n}                                                & PAD-inpaintBCT               & 83.72          & \textbf{89.94} & 86.08          & \textbf{73.58} & 74.61          & \textbf{79.43} & 84.67          & 75.70          & 67.57          \\
                                                                        & PAD-black                    & \textbf{87.53} & 87.69          & \textbf{88.92} & 70.73          & \textbf{74.84} & 78.68          & \textbf{85.37} & \textbf{81.51} & \textbf{77.25} \\ \hline
\end{tabular}%
}
\end{table*}

According to the results, inpaintBCT works better in some cases, but in most cases, black works better. Comparing the results in Table 1 of the main paper, it can be observed that regardless of the specific inpainting method used, both achieve superior defense performance compared to other state-of-the-art methods. This highlights the absolute advantage of PAD in patch localization, making the choice of inpainting method less crucial. The simplest removal method is sufficient to achieve a satisfactory defense effect.

%----------------------------------
% \subsection{More visualization examples}
% % 
% In Figure \ref{}, we present additional visual examples showcasing the patch localization process of PAD. These examples provide a broader coverage of PAD's performance in localizing various patches.

%=========================================================
\section{More About Evaluation on Physical Attacks}
%----------------------------------
\subsection{Ablation results on APRICOT}
To investigate the individual contributions of semantic independence and spatial heterogeneity in defense against physical attacks, we conducted ablation experiments on the APRICOT dataset. Table \ref{tab:apricot-ablation} presents the adversarial success rate (ASR) for five detectors using semantic independence alone, spatial heterogeneity alone, and both semantic independence and spatial heterogeneity combined.

\begin{table}[h]
\centering
\caption{ASR (\%) of ablated PAD on APRICOT. Lower values indicate better defense performance.}
\label{tab:apricot-ablation}
\resizebox{0.48\textwidth}{!}{%
\begin{tabular}{c|ccc}
\hline
Detector                                               & PAD-MI only   & PAD-CD only & PAD-all       \\ \hline
\begin{tabular}[c]{@{}c@{}}Faster\\ R-CNN\end{tabular} & {\ul 3.03}    & 4.54        & \textbf{2.27} \\ \hline
YOLOv2                                                 & {\ul 0.62}    & 1.52        & \textbf{0.43} \\ \hline
YOLOv3                                                 & \textbf{0}    & 0.64        & {\ul 0.60}    \\ \hline
YOLOv5s                                                & \textbf{0}    & \textbf{0}  & \textbf{0}    \\ \hline
YOLOv8n                                                & \textbf{0.27} & 0.45        & {\ul 0.42}    \\ \hline
\end{tabular}%
}
\end{table}

The experimental results indicate that under the physical attack setting, semantic independence performs better than spatial heterogeneity, yielding lower ASR values across all five detectors. This finding aligns with our analysis in Section 5.4 of the main paper. Even without adjusting the weights of semantic independence and spatial heterogeneity, PAD still achieves significant defense effectiveness.

%----------------------------------
\subsection{Visualization of patch localization on APRICOT}
In Figure \ref{fig:sup-apricot-vis}, we present visual examples showcasing the patch localization process of PAD on the APRICOT dataset. Compared with the visual examples under digital attacks in Figure 3 of the main paper, it can be observed that the influence of spatial heterogeneity in physical attack scenarios may be affected by lighting conditions, angles, and imaging processes. On the other hand, the significance of semantic independence becomes more prominent. These two characteristics play different roles in defending against digital and physical attacks, and their organic combination contributes to the exceptional performance of PAD.

Additionally, we compare the heat map when using semantic independence alone in PAD with the entropy-based defense approach \cite{tarchoun2023jedi} in Figure \ref{fig:sup-apricot-entro}. It can be observed that complex textured backgrounds, such as shelves filled with goods, have a significant impact on the entropy-based defense, resulting in high entropy values in a large portion of the background area. However, the performance of semantic independence localization based on mutual information in PAD, remains relatively stable. This is because although the background area is complex, adjacent regions still exhibit semantic correlation, leading to lower values of semantic independence.

\begin{figure*}[]
    \centering
    \includegraphics[width=1\textwidth]{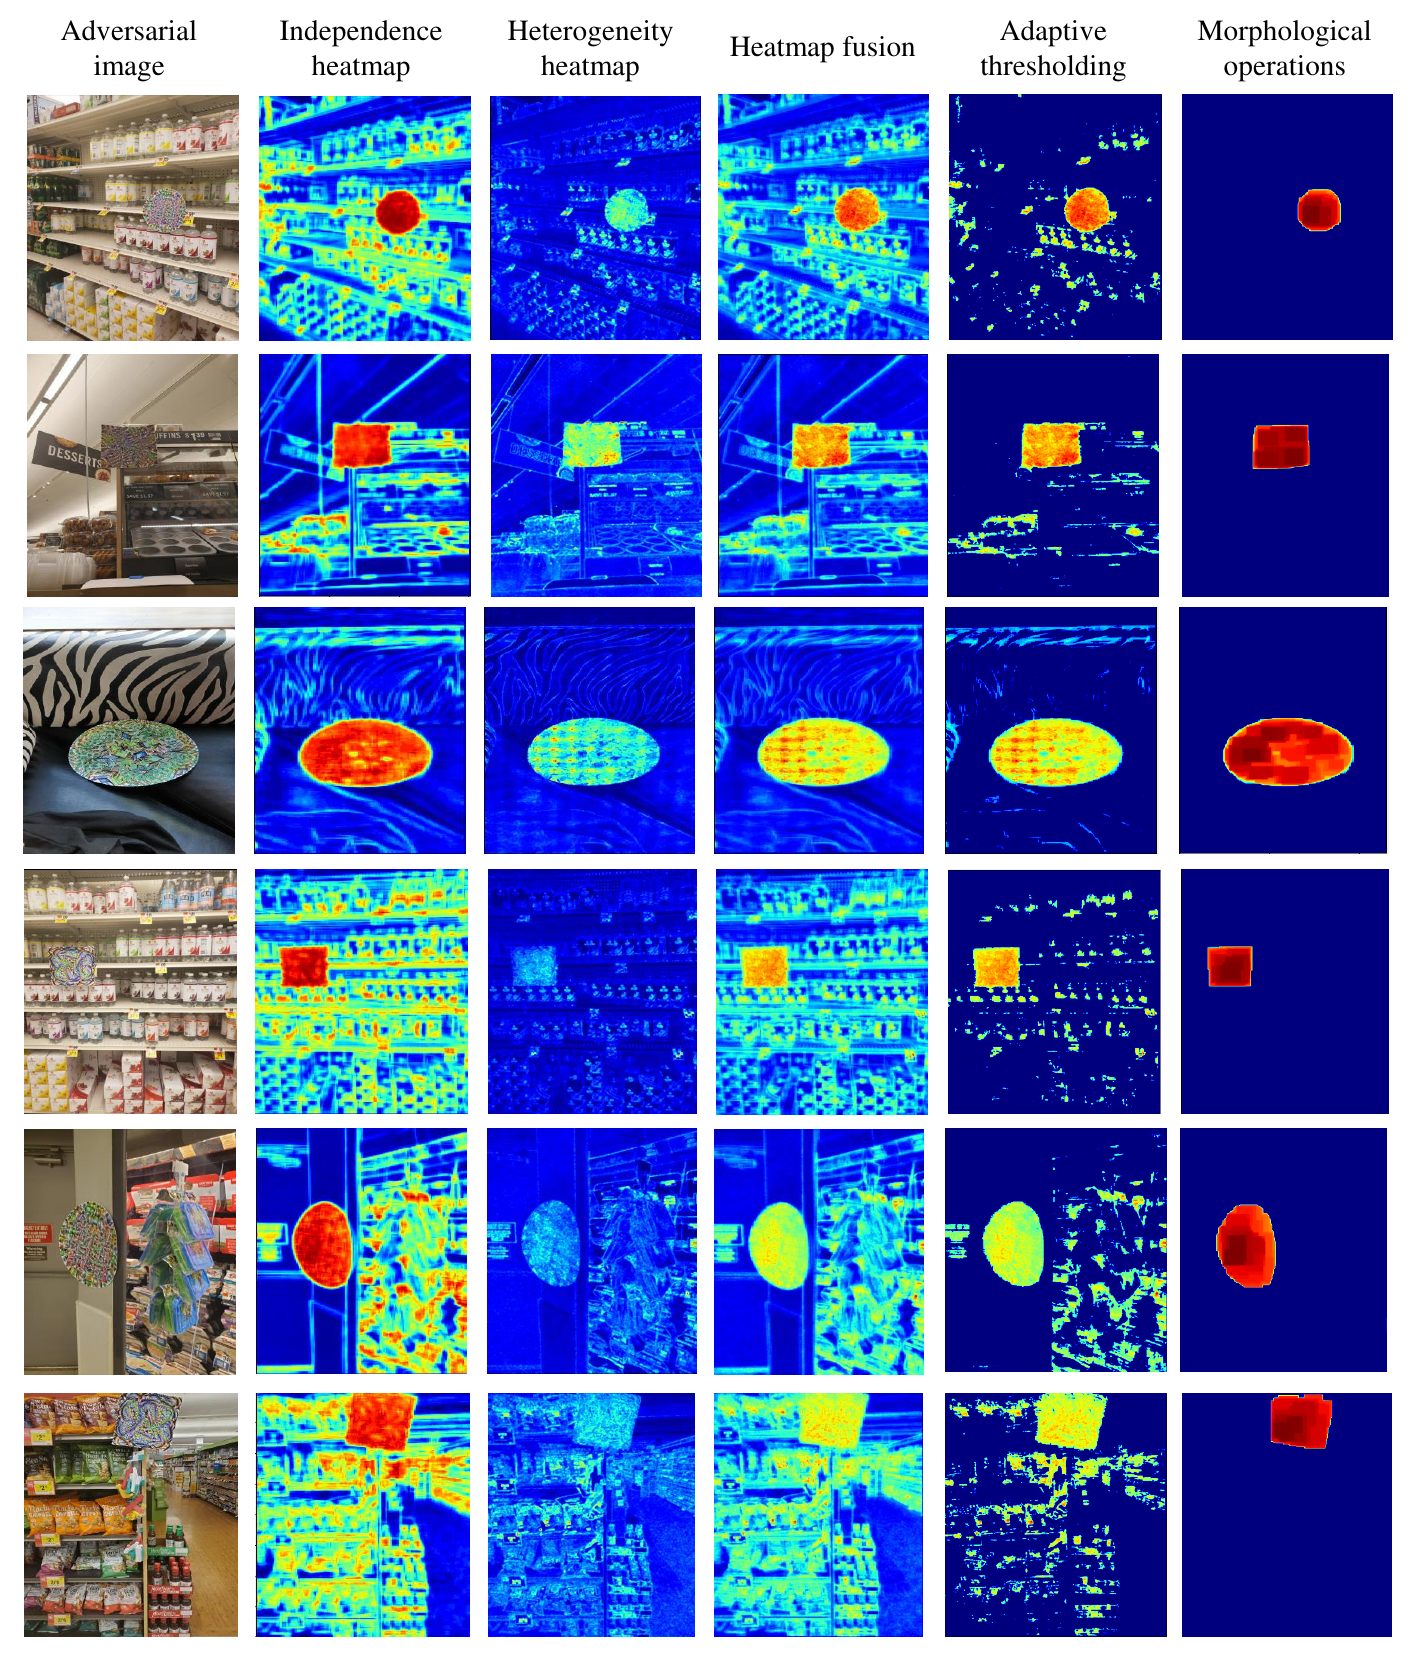}
    \caption{Visualization examples illustrating the patch localization process of PAD on APRICOT.}
    \label{fig:sup-apricot-vis}
\end{figure*}

\begin{figure*}[]
    \centering
    \includegraphics[width=1\textwidth]{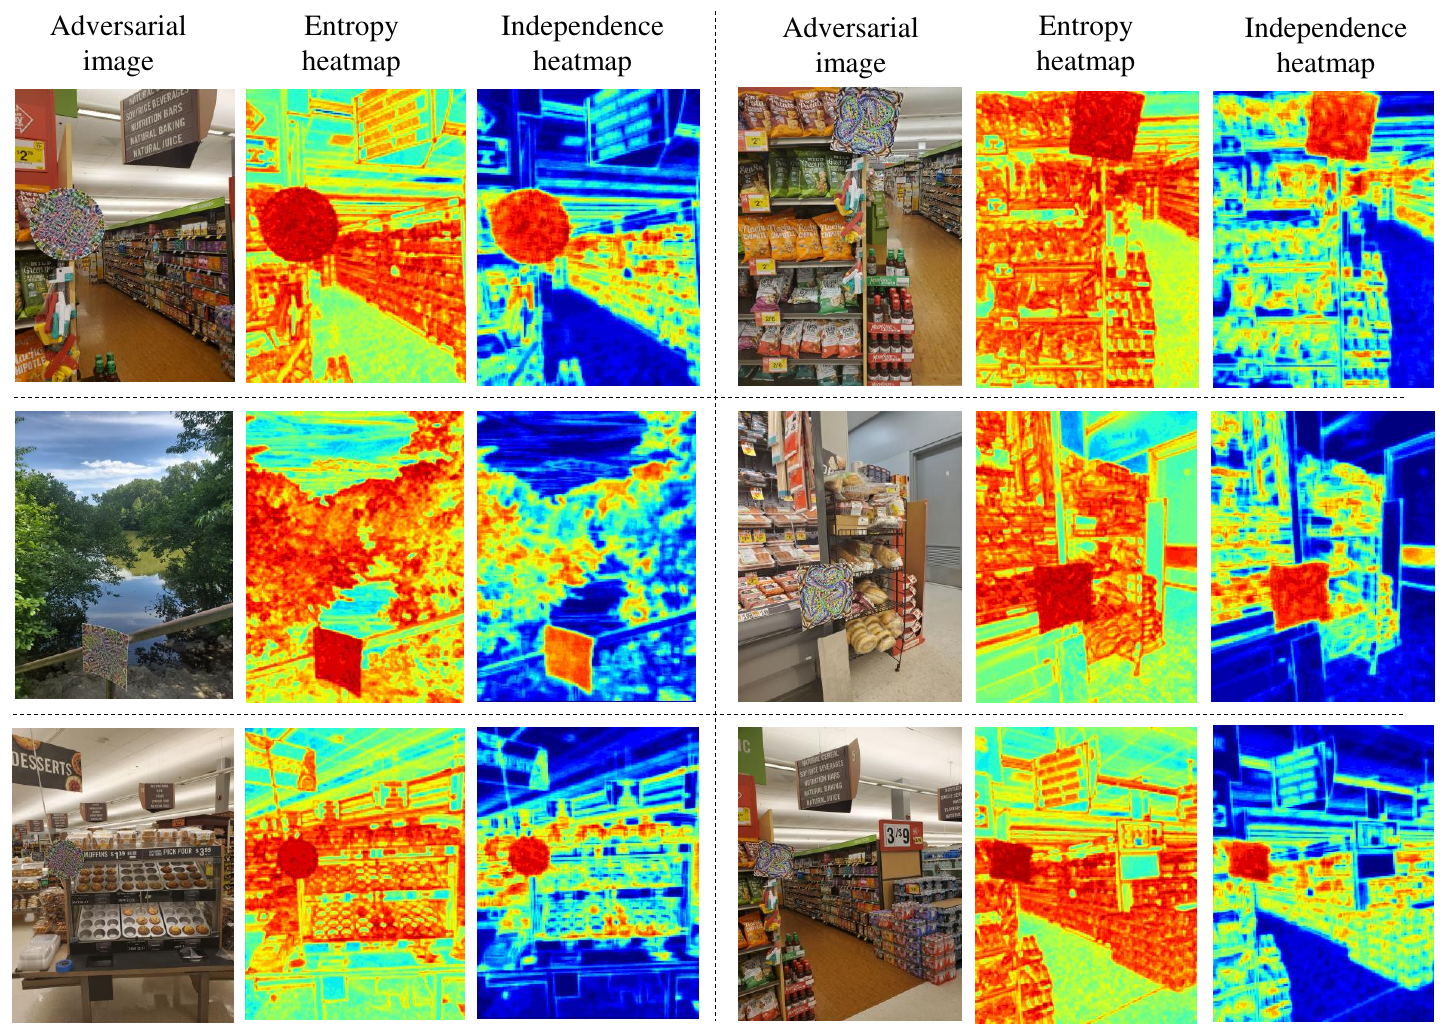}
    \caption{Visualization comparison of entropy heat map and semantic independence heat map.}
    \label{fig:sup-apricot-entro}
\end{figure*}

%----------------------------------
\subsection{Data distribution of physical test set}
\begin{figure}[h]
	\centering
	\begin{subfigure}{0.55\linewidth}
		\centering
		\includegraphics[width=0.9\linewidth]{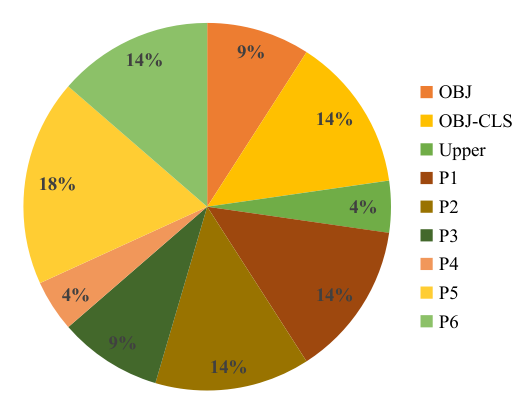}
		\caption{Adversarial patches}
		\label{physical-patch}
	\end{subfigure}
	\centering
	\begin{subfigure}{0.44\linewidth}
		\centering
		\includegraphics[width=0.9\linewidth]{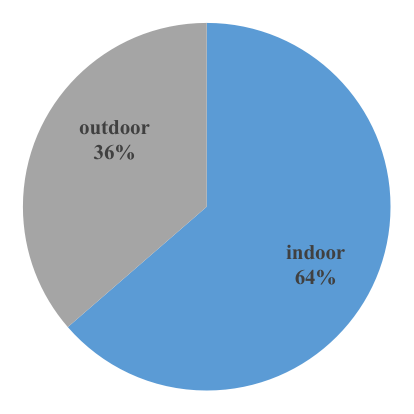}
		\caption{Scenes}
		\label{physical-indoor}
	\end{subfigure}
  \caption{Data distribution of our physical test set.}
  \label{fig:physical-distribution}	
\end{figure}

We print 9 different patches including P1-P6 \cite{hu2021naturalistic}, OBJ, OBJ-CLS, and Upper \cite{thys2019fooling}, taking videos in both indoor and outdoor environments across five different scenes. We build the physical test set which consists of 1100 images. Figure \ref{physical-patch} and Figure \ref{physical-indoor} display the distribution of the patches and indoor/outdoor scenes respectively.

%=========================================================
\section{Discussion on Adaptive Attacks}

In order to bypass the defense method proposed in this paper, attackers would need to ensure two key aspects during the patch generation process: 1) The image quality of the patch should be as consistent as possible with other parts of the image. 2) The patch should be semantically similar to its surrounding context. However, image quality can vary significantly depending on the capturing device and the image compression algorithms used. Additionally, the semantic content differs across each image and different positions within an image. Therefore, achieving both of these requirements would necessitate training unique patches for different positions within each image, rendering patch reusability impossible. This limitation proves fatal for physical attacks, meaning attackers cannot pre-train patches and simply print and place them in different scenes to execute attacks. Even if the goal is to target a fixed scene and angle, the presence of moving objects (such as pedestrians or vehicles) and the variability introduced by factors like camera angles and lighting condition would prevent the attacker from accurately predicting the final image composition. Additionally, if the patch content closely matches the surrounding semantic space, the detect model will likely confuse it with the surrounding context, resulting in a low probability of attack success. Therefore, the threat of adaptive attacks against PAD is weak.
